# Supplementary material for: A Mountaineering Strategy to Excited States: Revising Reference Values with EOM-CC4
Source: arXiv:2204.11658 source file (2022-06-07)
Supplement: Supplementary file 1 [file CC4-2-SI.pdf]

# A Mountaineering Strategy to Excited States: Exploring the EOM-CC4 Couloir: Supporting Information


Pierre-François Loos,[*,†] Filippo Lipparini,[‡] Devin A. Matthews,[¶] Aymeric Blondel,[§] and Denis Jacquemin[*,§]

†*Laboratoire de Chimie et Physique Quantiques, Université de Toulouse, CNRS, UPS, France*

‡*Dipartimento di Chimica e Chimica Industriale, University of Pisa, Via Moruzzi 3, 56124 Pisa, Italy*

¶*Department of Chemistry, Southern Methodist University, Dallas, Texas 75275, USA*

§*Université de Nantes, CNRS, CEISAM UMR 6230, F-44000 Nantes, France*

E-mail: loos@irsamc.ups-tlse.fr; Denis.Jacquemin@univ-nantes.fr

# S1 Raw benchmark data

Table S1: Vertical transition energies obtained with 6-31+G(d) for all systems containing two non-hydrogen atoms. We report the symmetry and the nature (valence or Rydberg) of the excited states. [F] stands for fluorescence, that is vertical emission rather than absorption. All values are in eV.

| Molecule | State | | CC2 | CCSD | CC3 | CCSDT | CC4 | CCSDTQ | CCSDTQP |
|---|---|---|---|---|---|---|---|---|---|
| Acetylene | $^1\Sigma_u^-(\pi \rightarrow \pi^*)$ | V | 7.502 | 7.493 | 7.404 | 7.410 | 7.406 | 7.402 | 7.402 |
| | $^1\Delta_u(\pi \rightarrow \pi^*)$ | V | 7.784 | 7.811 | 7.716 | 7.732 | 7.729 | 7.726 | 7.726 |
| | $^1A_u[F](\pi \rightarrow \pi^*)$ | V | 4.045 | 3.941 | 3.834 | 3.854 | 3.850 | 3.839 | 3.839 |
| | $^1A_2[F](\pi \rightarrow \pi^*)$ | V | 4.225 | 4.178 | 4.047 | 4.070 | 4.067 | 4.057 | 4.056 |
| Ethylene | $^1B_{3u}(\pi \rightarrow 3s)$ | R | 7.718 | 7.813 | 7.713 | 7.725 | 7.723 | 7.722 | 7.722 |
| | $^1B_{1u}(\pi \rightarrow \pi^*)$ | V | 8.123 | 8.275 | 8.142 | 8.152 | 8.138 | 8.137 | 8.135 |
| | $^1B_{1g}(\pi \rightarrow 3p)$ | R | 8.280 | 8.370 | 8.284 | 8.297 | 8.296 | 8.295 | 8.295 |
| Formaldehyde | $^1A_2(n \rightarrow \pi^*)$ | V | 4.151 | 4.031 | 4.031 | 4.011 | 4.021 | 4.022 | 4.023 |
| | $^1B_2(n \rightarrow 3s)$ | R | 6.649 | 7.238 | 7.241 | 7.232 | 7.279 | 7.279 | 7.287 |
| | $^1B_2(n \rightarrow 3p)$ | R | 7.501 | 7.994 | 8.019 | 8.007 | 8.044 | 8.045 | 8.051 |
| | $^1A_1(n \rightarrow 3p)$ | R | 7.695 | 8.282 | 8.305 | 8.295 | 8.342 | 8.341 | 8.350 |
| | $^1A_2(n \rightarrow 3p)$ | R | 8.156 | 8.666 | 8.703 | 8.682 | 8.723 | 8.724 | 8.732 |
| | $^1B_1(\sigma \rightarrow \pi^*)$ | V | 9.493 | 9.414 | 9.367 | 9.342 | 9.354 | 9.354 | 9.356 |
| | $^1A_1(\pi \rightarrow \pi^*)$ | V | 10.234 | 10.042 | 9.832 | 9.830 | 9.779 | 9.779 | 9.776 |
| | $^1A"[F](n \rightarrow \pi^*)$ | V | 3.029 | 2.916 | 2.880 | 2.850 | 2.860 | 2.862 | 2.863 |
| HCCl | $^1A"(\sigma \rightarrow \pi)$ | V | 1.974 | 2.054 | 2.048 | 2.045 | 2.052 | 2.052 | 2.053 |
| HCF | $^1A"(\sigma \rightarrow \pi)$ | V | 2.506 | 2.581 | 2.576 | 2.573 | 2.578 | 2.577 | 2.578 |
| HCP | $^1\Sigma^-(\pi \rightarrow \pi^*)$ | V | 5.326 | 5.242 | 5.191 | 5.187 | 5.181 | 5.176 | 5.175 |
| | $^1\Delta(\pi \rightarrow \pi^*)$ | V | 5.680 | 5.535 | 5.478 | 5.485 | 5.481 | 5.476 | 5.476 |
| HPO | $^1A''(n \rightarrow \pi^*)$ | V | 2.525 | 2.526 | 2.492 | 2.474 | 2.481 | 2.481 | 2.483 |
| HPS | $^1A''(n \rightarrow \pi^*)$ | V | 1.667 | 1.616 | 1.566 | 1.553 | 1.555 | 1.555 | 1.555 |
| HSiF | $^1A''(\sigma \rightarrow \pi)$ | V | 3.169 | 3.139 | 3.094 | 3.080 | 3.080 | 3.079 | 3.080 |
| Methanimine | $^1A"(n \rightarrow \pi^*)$ | V | 5.483 | 5.391 | 5.338 | 5.323 | 5.326 | 5.327 | 5.327 |
| Nitroxyl | $^1A''(n \rightarrow \pi^*)$ | V | 1.798 | 1.802 | 1.806 | 1.796 | 1.799 | 1.799 | 1.800 |
| | $^1A'(n, n \rightarrow \pi^*, \pi^*)$ | V | | | 5.278 | 4.819 | 4.562 | 4.535 | 4.513 |
| | $^1A'(n.d.)$ | R | 6.106 | 6.594 | 6.600 | 6.593 | 6.603 | 6.609 | 6.612 |
| Silylidene | $^1A_2(n.d.)$ | | 2.360 | 2.254 | 2.141 | 2.107 | 2.100 | 2.101 | 2.101 |
| | $^1B_2(n.d.)$ | | 3.925 | 3.966 | 3.878 | 3.874 | 3.873 | 3.876 | 3.877 |
| Thioformaldehyde | $^1A_2(n \rightarrow \pi^*)$ | V | 2.397 | 2.302 | 2.262 | 2.244 | 2.246 | 2.246 | 2.247 |
| | $^1B_2(n \rightarrow 4s)$ | R | 5.848 | 5.937 | 5.878 | 5.875 | 5.884 | 5.890 | 5.893 |
| | $^1A_1(\pi \rightarrow \pi^*)$ | V | 6.955 | 6.961 | 6.817 | 6.790 | 6.723 | 6.713 | 6.708 |
| | $^1A_2[F](n \rightarrow \pi^*)$ | V | 2.134 | 2.040 | 1.988 | 1.964 | 1.967 | 1.967 | 1.968 |

Table S2: Vertical transition energies obtained with *aug*-cc-pVDZ for all systems containing two non-hydrogen atoms. See Table S1 for more details.

| Molecule | State | | CC2 | CCSD | CC3 | CCSDT | CC4 | CCSDTQ |
|---|---|---|---|---|---|---|---|---|
| Acetylene | $^1\Sigma_u^-(\pi \rightarrow \pi^*)$ | V | 7.319 | 7.270 | 7.207 | 7.211 | 7.210 | 7.206 |
| | $^1\Delta_u(\pi \rightarrow \pi^*)$ | V | 7.634 | 7.566 | 7.507 | 7.519 | 7.521 | 7.517 |
| | $^1A_u[F](\pi \rightarrow \pi^*)$ | V | 3.939 | 3.777 | 3.697 | 3.718 | 3.715 | 3.705 |
| | $^1A_2[F](\pi \rightarrow \pi^*)$ | V | 4.127 | 4.016 | 3.917 | 3.939 | 3.939 | 3.929 |
| Ethylene | $^1B_{3u}(\pi \rightarrow 3s)$ | R | 7.170 | 7.323 | 7.286 | 7.294 | 7.304 | 7.303 |
| | $^1B_{1u}(\pi \rightarrow \pi^*)$ | V | 7.916 | 8.035 | 7.935 | 7.944 | 7.933 | 7.932 |
| | $^1B_{1g}(\pi \rightarrow 3p)$ | R | 7.840 | 8.003 | 7.974 | 7.984 | 7.993 | 7.992 |
| Formaldehyde | $^1A_2(n \rightarrow \pi^*)$ | V | 4.092 | 4.020 | 4.003 | 3.986 | 3.996 | 3.997 |
| | $^1B_2(n \rightarrow 3s)$ | R | 6.397 | 7.043 | 7.051 | 7.040 | 7.094 | 7.091 |
| | $^1B_2(n \rightarrow 3p)$ | R | 7.477 | 7.993 | 8.017 | 8.002 | 8.047 | 8.045 |
| | $^1A_1(n \rightarrow 3p)$ | R | 7.384 | 8.052 | 8.081 | 8.068 | 8.123 | 8.119 |
| | $^1A_2(n \rightarrow 3p)$ | R | 8.061 | 8.614 | 8.655 | 8.630 | 8.680 | 8.678 |
| | $^1B_1(\sigma \rightarrow \pi^*)$ | V | 9.419 | 9.373 | 9.309 | 9.288 | 9.304 | 9.302 |
| | $^1A_1(\pi \rightarrow \pi^*)$ | V | 9.638 | 9.752 | 9.590 | 9.588 | 9.544 | 9.544 |
| | $^1A"[F](n \rightarrow \pi^*)$ | V | 2.989 | 2.924 | 2.872 | 2.844 | 2.854 | 2.855 |
| HCCl | $^1A"(\sigma \rightarrow \pi)$ | V | 1.958 | 2.035 | 2.022 | 2.018 | 2.025 | 2.025 |
| HCF | $^1A"(\sigma \rightarrow \pi)$ | V | 2.465 | 2.541 | 2.533 | 2.529 | 2.534 | 2.533 |
| HCP | $^1\Sigma^-(\pi \rightarrow \pi^*)$ | V | 5.219 | 5.085 | 5.058 | 5.054 | 5.049 | 5.044 |
| | $^1\Delta(\pi \rightarrow \pi^*)$ | V | 5.543 | 5.350 | 5.325 | 5.330 | 5.329 | 5.324 |
| HPO | $^1A''(n \rightarrow \pi^*)$ | V | 2.478 | 2.515 | 2.465 | 2.452 | 2.460 | 2.459 |
| HPS | $^1A''(n \rightarrow \pi^*)$ | V | 1.677 | 1.668 | 1.601 | 1.589 | 1.590 | 1.590 |
| HSiF | $^1A''(\sigma \rightarrow \pi)$ | V | 3.138 | 3.120 | 3.077 | 3.066 | 3.066 | 3.065 |
| Methanimine | $^1A"(n \rightarrow \pi^*)$ | V | 5.376 | 5.316 | 5.257 | 5.242 | 5.245 | 5.245 |
| Nitroxyl | $^1A''(n \rightarrow \pi^*)$ | V | 1.765 | 1.779 | 1.777 | 1.767 | 1.769 | 1.770 |
| | $^1A'(n, n \rightarrow \pi^*, \pi^*)$ | V | | | 5.247 | 4.756 | 4.454 | 4.424 |
| | $^1A'(n.d.)$ | R | 5.557 | 6.117 | 6.123 | 6.115 | 6.132 | 6.136 |
| Silylidene | $^1A_2(n.d.)$ | | 2.379 | 2.289 | 2.179 | 2.146 | 2.139 | 2.140 |
| | $^1B_2(n.d.)$ | | 3.857 | 3.875 | 3.802 | 3.795 | 3.796 | 3.798 |
| Thioformaldehyde | $^1A_2(n \rightarrow \pi^*)$ | V | 2.387 | 2.325 | 2.272 | 2.253 | 2.255 | 2.255 |
| | $^1B_2(n \rightarrow 4s)$ | R | 5.699 | 5.841 | 5.801 | 5.796 | 5.812 | 5.816 |
| | $^1A_1(\pi \rightarrow \pi^*)$ | V | 6.664 | 6.749 | 6.617 | 6.597 | 6.524 | 6.512 |
| | $^1A_2[F](n \rightarrow \pi^*)$ | V | 2.126 | 2.072 | 2.004 | 1.980 | 1.982 | 1.982 |

Table S3: Vertical transition energies obtained with *aug*-cc-pVTZ for all systems containing two non-hydrogen atoms. See Table S1 for more details.

| Molecule | State | | CC2 | CCSD | CC3 | CCSDT | CC4 | CCSDTQ |
|---|---|---|---|---|---|---|---|---|
| Acetylene | $^1\Sigma_u^-(\pi \to \pi^*)$ | V | 7.260 | 7.150 | 7.089 | 7.095 | 7.086 | 7.084 |
| | $^1\Delta_u(\pi \to \pi^*)$ | V | 7.594 | 7.480 | 7.421 | 7.435 | 7.429 | 7.428 |
| | $^1A_u[F](\pi \to \pi^*)$ | V | 3.936 | 3.703 | 3.640 | 3.659 | 3.649 | 3.642 |
| | $^1A_2[F](\pi \to \pi^*)$ | V | 4.108 | 3.925 | 3.839 | 3.861 | 3.852 | 3.845 |
| Ethylene | $^1B_{3u}(\pi \to 3s)$ | R | 7.293 | 7.417 | 7.354 | 7.365 | 7.368 | 7.367 |
| | $^1B_{1u}(\pi \to \pi^*)$ | V | 7.925 | 8.020 | 7.905 | 7.918 | 7.899 | 7.899 |
| | $^1B_{1g}(\pi \to 3p)$ | R | 7.947 | 8.078 | 8.025 | 8.037 | 8.039 | 8.039 |
| Formaldehyde | $^1A_2(n \to \pi^*)$ | V | 4.072 | 4.013 | 3.971 | 3.954 | 3.965 | 3.965 |
| | $^1B_2(n \to 3s)$ | R | 6.558 | 7.231 | 7.179 | 7.165 | 7.219 | 7.213 |
| | $^1B_2(n \to 3p)$ | R | 7.568 | 8.120 | 8.086 | 8.070 | 8.114 | 8.110 |
| | $^1A_1(n \to 3p)$ | R | 7.518 | 8.210 | 8.182 | 8.164 | 8.219 | 8.213 |
| | $^1A_2(n \to 3p)$ | R | 8.043 | 8.650 | 8.636 | 8.609 | 8.659 | 8.655 |
| | $^1B_1(\sigma \to \pi^*)$ | V | 9.322 | 9.281 | 9.190 | 9.173 | 9.187 | 9.185 |
| | $^1A_1(\pi \to \pi^*)$ | V | 9.537 | 9.670 | 9.482 | 9.488 | 9.434 | 9.435 |
| | $^1A"[F](n \to \pi^*)$ | V | 2.973 | 2.928 | 2.844 | 2.819 | 2.829 | 2.829 |
| HCCl | $^1A"(\sigma \to \pi)$ | V | 1.912 | 1.987 | 1.971 | 1.967 | 1.974 | 1.974 |
| HCF | $^1A"(\sigma \to \pi)$ | V | 2.436 | 2.507 | 2.496 | 2.493 | 2.498 | 2.497 |
| HCP | $^1\Sigma^-(\pi \to \pi^*)$ | V | 5.075 | 4.868 | 4.850 | 4.845 | 4.838 | 4.835 |
| | $^1\Delta(\pi \to \pi^*)$ | V | 5.406 | 5.162 | 5.147 | 5.152 | 5.148 | 5.145 |
| HPO | $^1A''(n \to \pi^*)$ | V | 2.495 | 2.539 | 2.465 | 2.455 | 2.462 | 2.461 |
| HPS | $^1A''(n \to \pi^*)$ | V | 1.678 | 1.673 | 1.591 | 1.580 | 1.578 | 1.579 |
| HSiF | $^1A''(\sigma \to \pi)$ | V | 3.143 | 3.120 | 3.070 | 3.060 | 3.058 | 3.058 |
| Methanimine | $^1A"(n \to \pi^*)$ | V | 5.324 | 5.278 | 5.203 | 5.190 | 5.192 | 5.193 |
| Nitroxyl | $^1A''(n \to \pi^*)$ | V | 1.741 | 1.756 | 1.747 | 1.737 | 1.742 | 1.742 |
| | $^1A'(n,n \to \pi^*,\pi^*)$ | V | | | 5.257 | 4.785 | 4.380 | 4.364 |
| | $^1A'(n.d.)$ | R | 5.718 | 6.310 | 6.256 | 6.249 | 6.265 | 6.268 |
| Silylidene | $^1A_2(n.d.)$ | | 2.366 | 2.286 | 2.154 | 2.128 | 2.116 | 2.118 |
| | $^1B_2(n.d.)$ | | 3.852 | 3.877 | 3.780 | 3.779 | 3.776 | 3.779 |
| Thioformaldehyde | $^1A_2(n \to \pi^*)$ | V | 2.339 | 2.291 | 2.228 | 2.207 | 2.208 | 2.208 |
| | $^1B_2(n \to 4s)$ | R | 5.815 | 5.970 | 5.910 | 5.900 | 5.912 | 5.914 |
| | $^1A_1(\pi \to \pi^*)$ | V | 6.708 | 6.633 | 6.484 | 6.467 | 6.372 | 6.360 |
| | $^1A_2[F](n \to \pi^*)$ | V | 2.087 | 2.050 | 1.969 | 1.943 | 1.945 | 1.944 |

Table S4: Vertical transition energies obtained with 6-31+G(d) for all systems containing three non-hydrogen atoms. See Table S1 for more details.

| Molecule | State | | CC2 | CCSD | CC3 | CCSDT | CC4 | CCSDTQ |
|---|---|---|---|---|---|---|---|---|
| Acetaldehyde | $^1A''(n \to \pi^*)$ | V | 4.507 | 4.396 | 4.393 | 4.367 | 4.376 | 4.376 |
| $CCl_2$ | $^1B_1(\sigma \to \pi)$ | V | 2.664 | 2.697 | 2.706 | 2.696 | 2.704 | 2.704 |
| | $^1A_2(n.d.)$ | V | 4.386 | 4.633 | 4.467 | 4.442 | 4.482 | 4.475 |
| CClF | $^1A"(\sigma \to \pi)$ | V | 3.662 | 3.673 | 3.664 | 3.656 | 3.660 | 3.660 |
| $CF_2$ | $^1B_1(\sigma \to \pi)$ | V | 5.173 | 5.191 | 5.183 | 5.178 | 5.181 | 5.180 |
| Cyclopropene | $^1B_1(\sigma \to \pi)$ | V | 6.911 | 6.926 | 6.855 | 6.847 | 6.842 | 6.841 |
| | $^1B_2(\pi \to \pi^*)$ | V | 7.015 | 7.107 | 6.980 | 6.990 | 6.979 | 6.978 |
| Diazirine | $^1B_1(n \to \pi^*)$ | V | 4.299 | 4.279 | 4.196 | 4.185 | 4.174 | 4.173 |
| | $^1A_2(n \to 3s)$ | R | 7.583 | 7.512 | 7.432 | 7.400 | 7.392 | 7.390 |
| | $^1B_2(\sigma \to \pi)$ | V | 7.486 | 7.730 | 7.623 | 7.617 | 7.603 | 7.606 |
| | $^1A_1(n \to 3p)$ | R | 7.839 | 8.121 | 8.048 | 8.032 | 8.021 | 8.023 |
| Diazomethane | $^1A_2(\pi \to \pi^*)$ | V | 3.383 | 3.186 | 3.051 | 3.045 | 3.028 | 3.027 |
| | $^1B_1(\pi \to 3s)$ | R | 5.499 | 5.507 | 5.367 | 5.395 | 5.371 | 5.375 |
| | $^1A_1(\pi \to \pi^*)$ | V | 6.038 | 5.953 | 5.833 | 5.856 | 5.819 | 5.824 |
| | $^1A''[F](\pi \to \pi^*)$ | V | 0.864 | 0.751 | 0.617 | 0.603 | 0.587 | 0.587 |
| Formamide | $^1A''(n \to \pi^*)$ | V | 5.883 | 5.802 | 5.827 | 5.792 | 5.808 | 5.808 |
| | $^1A'(n \to 3s)$ | R | 6.477 | 7.053 | 6.854 | 6.846 | 6.867 | 6.860 |
| Formylfluoride | $^1A''(n \to \pi^*)$ | V | 6.263 | 6.073 | 6.094 | 6.062 | 6.071 | 6.072 |
| Ketene | $^1A_2(\pi \to \pi^*)$ | V | 4.191 | 3.955 | 3.864 | 3.853 | 3.838 | 3.840 |
| | $^1B_1(n \to 3s)$ | R | 5.937 | 6.042 | 5.907 | 5.938 | 5.931 | 5.934 |
| | $^1A_1(\pi \to \pi^*)$ | V | 7.370 | 7.427 | 7.316 | 7.335 | 7.329 | 7.331 |
| | $^1A_2(\pi \to 3p)$ | R | 7.327 | 7.471 | 7.340 | 7.380 | 7.374 | 7.377 |
| | $^1A"[F](\pi \to \pi^*)$ | V | 1.197 | 1.039 | 0.904 | 0.900 | 0.877 | 0.900 |
| Nitrosomethane | $^1A''(n \to \pi^*)$ | V | 2.028 | 2.015 | 2.018 | 2.003 | 2.004 | 2.004 |
| | $^1A'(n, n \to \pi^*, \pi^*)$ | V | | | 5.729 | 5.260 | 4.926 | 4.895 |
| | $^1A'(n.d.)$ | R | 6.064 | 6.551 | 6.486 | 6.479 | 6.485 | 6.489 |
| | $^1A''[F](n \to \pi^*)$ | V | 1.713 | 1.714 | 1.719 | 1.704 | 1.706 | 1.707 |
| $SiCl_2$ | $^1B_1(\sigma \to \pi)$ | V | 4.030 | 4.009 | 3.949 | 3.940 | 3.940 | 3.939 |
| Steptocyanine-1 | $^1B_2(\pi \to \pi^*)$ | V | 7.380 | 7.355 | 7.278 | 7.254 | 7.257 | 7.260 |

Table S5: Vertical transition energies obtained with *aug*-cc-pVDZ for all systems containing three non-hydrogen atoms. See Table S1 for more details.

| Molecule | State | | CC2 | CCSD | CC3 | CCSDT | CC4 | CCSDTQ |
|---|---|---|---|---|---|---|---|---|
| Acetaldehyde | $^1A''(n \rightarrow \pi^*)$ | V | 4.434 | 4.364 | 4.344 | 4.321 | 4.332 | 4.332 |
| $CCl_2$ | $^1B_1(\sigma \rightarrow \pi)$ | V | 2.671 | 2.695 | 2.696 | 2.685 | 2.693 | 2.693 |
| | $^1A_2(n.d.)$ | V | 4.316 | 4.577 | 4.405 | 4.385 | 4.422 | 4.413 |
| CClF | $^1A"(\sigma \rightarrow \pi)$ | V | 3.643 | 3.642 | 3.631 | 3.621 | 3.626 | 3.625 |
| $CF_2$ | $^1B_1(\sigma \rightarrow \pi)$ | V | 5.130 | 5.131 | 5.116 | 5.109 | 5.110 | 5.110 |
| Cyclopropene | $^1B_1(\sigma \rightarrow \pi)$ | V | 6.691 | 6.777 | 6.720 | 6.711 | 6.711 | 6.710 |
| | $^1B_2(\pi \rightarrow \pi^*)$ | V | 6.786 | 6.876 | 6.771 | 6.779 | 6.772 | 6.770 |
| Diazirine | $^1B_1(n \rightarrow \pi^*)$ | V | 4.254 | 4.238 | 4.164 | 4.153 | 4.142 | 4.142 |
| | $^1A_2(n \rightarrow 3s)$ | R | 7.535 | 7.478 | 7.396 | 7.366 | 7.358 | 7.356 |
| | $^1B_2(\sigma \rightarrow \pi)$ | V | 7.117 | 7.421 | 7.361 | 7.351 | 7.349 | 7.350 |
| | $^1A_1(n \rightarrow 3p)$ | R | 7.723 | 8.017 | 7.972 | 7.954 | 7.951 | 7.952 |
| Diazomethane | $^1A_2(\pi \rightarrow \pi^*)$ | V | 3.407 | 3.227 | 3.102 | 3.097 | 3.080 | 3.079 |
| | $^1B_1(\pi \rightarrow 3s)$ | R | 5.378 | 5.423 | 5.323 | 5.350 | 5.335 | 5.338 |
| | $^1A_1(\pi \rightarrow \pi^*)$ | V | 5.972 | 5.898 | 5.802 | 5.822 | 5.790 | 5.794 |
| | $^1A''[F](\pi \rightarrow \pi^*)$ | V | 0.908 | 0.812 | 0.682 | 0.668 | 0.651 | 0.651 |
| Formamide | $^1A''(n \rightarrow \pi^*)$ | V | 5.734 | 5.710 | 5.710 | 5.678 | 5.697 | 5.695 |
| | $^1A'(n \rightarrow 3s)$ | R | 6.165 | 6.833 | 6.646 | 6.639 | 6.674 | 6.664 |
| Formylfluoride | $^1A''(n \rightarrow \pi^*)$ | V | 6.182 | 6.031 | 6.034 | 6.003 | 6.015 | 6.015 |
| Ketene | $^1A_2(\pi \rightarrow \pi^*)$ | V | 4.190 | 3.974 | 3.892 | 3.882 | 3.868 | 3.869 |
| | $^1B_1(n \rightarrow 3s)$ | R | 5.786 | 5.938 | 5.832 | 5.862 | 5.862 | 5.864 |
| | $^1A_1(\pi \rightarrow \pi^*)$ | V | 7.267 | 7.336 | 7.242 | 7.258 | 7.255 | 7.256 |
| | $^1A_2(\pi \rightarrow 3p)$ | R | 6.939 | 7.148 | 7.049 | 7.088 | 7.090 | 7.093 |
| | $^1A"[F](\pi \rightarrow \pi^*)$ | V | 1.268 | 1.125 | 0.997 | 0.991 | 0.967 | 0.969 |
| Nitrosomethane | $^1A''(n \rightarrow \pi^*)$ | V | 2.004 | 2.001 | 1.998 | 1.984 | 1.985 | 1.985 |
| | $^1A'(n, n \rightarrow \pi^*, \pi^*)$ | V | | | 5.749 | 5.258 | 4.878 | 4.848 |
| | $^1A'(n.d.)$ | R | 5.695 | 6.257 | 6.197 | 6.189 | 6.207 | 6.209 |
| | $^1A''[F](n \rightarrow \pi^*)$ | V | 1.690 | 1.700 | 1.701 | 1.687 | 1.689 | 1.690 |
| $SiCl_2$ | $^1B_1(\sigma \rightarrow \pi)$ | V | 4.017 | 3.987 | 3.929 | 3.918 | 3.918 | 3.918 |
| Steptocyanine-1 | $^1B_2(\pi \rightarrow \pi^*)$ | V | 7.223 | 7.218 | 7.138 | 7.116 | 7.118 | 7.121 |

Table S6: Vertical transition energies obtained with *aug*-cc-pVTZ for all systems containing three non-hydrogen atoms. See Table S1 for more details.

| Molecule | State | | CC2 | CCSD | CC3 | CCSDT | CC4 |
|---|---|---|---|---|---|---|---|
| Acetaldehyde | $^1A''(n \to \pi^*)$ | V | 4.412 | 4.362 | 4.314 | 4.293 | |
| $CCl_2$ | $^1B_1(\sigma \to \pi)$ | V | 2.584 | 2.607 | 2.608 | 2.596 | 2.605 |
| | $^1A_2(n.d.)$ | V | 4.274 | 4.568 | 4.349 | 4.333 | 4.362 |
| CClF | $^1A"(\sigma \to \pi)$ | V | 3.571 | 3.572 | 3.560 | 3.550 | 3.554 |
| $CF_2$ | $^1B_1(\sigma \to \pi)$ | V | 5.086 | 5.091 | 5.069 | 5.064 | 5.066 |
| Cyclopropene | $^1B_1(\sigma \to \pi)$ | V | 6.730 | 6.764 | 6.683 | 6.676 | 6.673 |
| | $^1B_2(\pi \to \pi^*)$ | V | 6.785 | 6.856 | 6.733 | 6.746 | 6.731 |
| Diazirine | $^1B_1(n \to \pi^*)$ | V | 4.204 | 4.184 | 4.114 | 4.105 | 4.109 |
| | $^1A_2(n \to 3s)$ | R | 7.454 | 7.391 | 7.307 | 7.283 | 7.286 |
| | $^1B_2(\sigma \to \pi)$ | V | 7.257 | 7.554 | 7.450 | 7.448 | 7.437 |
| | $^1A_1(n \to 3p)$ | R | 7.808 | 8.115 | 8.037 | 8.026 | 8.017 |
| Diazomethane | $^1A_2(\pi \to \pi^*)$ | V | 3.367 | 3.191 | 3.070 | 3.068 | 3.048 |
| | $^1B_1(\pi \to 3s)$ | R | 5.528 | 5.570 | 5.451 | 5.483 | 5.461 |
| | $^1A_1(\pi \to \pi^*)$ | V | 6.002 | 5.943 | 5.836 | 5.859 | 5.823 |
| | $^1A''[F](\pi \to \pi^*)$ | V | 0.903 | 0.809 | 0.678 | 0.668 | 0.647 |
| Formamide | $^1A''(n \to \pi^*)$ | V | 5.689 | 5.692 | 5.657 | 5.627 | |
| | $^1A'(n \to 3s)$ | R | 6.311 | 6.992 | 6.743 | 6.741 | |
| Formylfluoride | $^1A''(n \to \pi^*)$ | V | 6.146 | 6.016 | 5.988 | 5.960 | 5.972 |
| Ketene | $^1A_2(\pi \to \pi^*)$ | V | 4.165 | 3.970 | 3.882 | 3.874 | 3.859 |
| | $^1B_1(n \to 3s)$ | R | 5.942 | 6.093 | 5.956 | 5.992 | 5.985 |
| | $^1A_1(\pi \to \pi^*)$ | V | 7.260 | 7.356 | 7.231 | 7.254 | 7.246 |
| | $^1A_2(\pi \to 3p)$ | R | 7.086 | 7.292 | 7.157 | 7.203 | 7.200 |
| | $^1A^"[F](\pi \to \pi^*)$ | V | 1.263 | 1.134 | 0.999 | 0.997 | 0.970 |
| Nitrosomethane | $^1A''(n \to \pi^*)$ | V | 1.978 | 1.976 | 1.965 | 1.951 | |
| | $^1A'(n, n \to \pi^*, \pi^*)$ | V | | | 5.757 | 5.293 | |
| | $^1A'(n.d.)$ | R | 5.841 | 6.435 | 6.310 | 6.304 | |
| | $^1A''[F](n \to \pi^*)$ | V | 1.668 | 1.677 | 1.670 | 1.657 | |
| $SiCl_2$ | $^1B_1(\sigma \to \pi)$ | V | 3.991 | 3.964 | 3.896 | 3.884 | 3.883 |
| Steptocyanine-1 | $^1B_2(\pi \to \pi^*)$ | V | 7.202 | 7.242 | 7.126 | 7.110 | |

Table S7: Vertical transition energies obtained with 6-31+G(d) for all systems containing four non-hydrogen atoms. See Table S1 for more details.

| Molecule | State | | CC2 | CCSD | CC3 | CCSDT | CC4 | CCSDTQ |
|---|---|---|---|---|---|---|---|---|
| Acetone | $^1A_2(n \to \pi^*)$ | V | 4.637 | 4.563 | 4.553 | 4.522 | 4.532 | 4.532 |
| | $^1B_2(n \to 3s)$ | R | 6.199 | 6.751 | 6.647 | 6.644 | 6.688 | 6.682 |
| | $^1A_2(n \to 3p)$ | R | 7.328 | 7.914 | 7.834 | 7.830 | 7.877 | 7.872 |
| | $^1A_1(n \to 3p)$ | R | 7.316 | 7.934 | 7.806 | 7.808 | 7.850 | 7.845 |
| | $^1B_2(n \to 3p)$ | R | 7.383 | 7.914 | 7.868 | 7.868 | 7.910 | 7.905 |
| Acrolein | $^1A''(n \to \pi^*)$ | V | 3.947 | 3.940 | 3.826 | 3.796 | 3.799 | 3.798 |
| | $^1A'(\pi \to \pi^*)$ | V | 6.984 | 7.047 | 6.832 | 6.862 | 6.835 | 6.836 |
| | $^1A''(n \to \pi^*)$ | V | 6.893 | 7.398 | 6.943 | 6.885 | 6.839 | 6.824 |
| | $^1A'(n \to 3s)$ | R | 6.576 | 7.325 | 7.222 | 7.231 | 7.263 | 7.260 |
| Butadiene | $^1B_u(\pi \to \pi^*)$ | V | 6.322 | 6.549 | 6.414 | 6.429 | 6.413 | 6.411 |
| | $^1B_g(\pi \to 3s)$ | R | 6.527 | 6.644 | 6.535 | 6.554 | 6.545 | 6.545 |
| | $^1A_g(\pi \to \pi^*)$ | V | 7.262 | 7.120 | 6.730 | 6.632 | 6.558 | 6.556 |
| | $^1A_u(\pi \to 3p)$ | R | 6.868 | 6.976 | 6.868 | 6.887 | 6.879 | 6.878 |
| | $^1A_u(\pi \to 3p)$ | R | 6.897 | 7.047 | 6.931 | 6.951 | 6.943 | 6.942 |
| | $^1B_u(\pi \to 3p)$ | R | 7.988 | 8.109 | 7.984 | 8.000 | 7.986 | 7.986 |
| Carbonylfluoride | $^1A_2(n \to \pi^*)$ | V | 7.481 | 7.331 | 7.332 | 7.300 | 7.311 | 7.311 |
| Cyanoacetylene | $^1\Sigma^-(\pi \to \pi^*)$ | V | 6.197 | 6.111 | 6.025 | 6.034 | 6.021 | 6.017 |
| | $^1\Delta(\pi \to \pi^*)$ | V | 6.470 | 6.379 | 6.290 | 6.306 | 6.296 | 6.293 |
| | $^1A''[F](\pi \to \pi^*)$ | V | 3.876 | 3.756 | 3.703 | 3.722 | 3.708 | 3.700 |
| Cyanoformaldehyde | $^1A''(n \to \pi^*)$ | V | 4.061 | 3.970 | 3.914 | 3.889 | 3.891 | 3.892 |
| | $^1A''(\pi \to \pi^*)$ | V | 6.941 | 6.898 | 6.636 | 6.672 | 6.640 | 6.640 |
| Cyanogen | $^1\Sigma_u^-(\pi \to \pi^*)$ | V | 6.893 | 6.732 | 6.617 | 6.626 | 6.615 | 6.610 |
| | $^1\Delta_u(\pi \to \pi^*)$ | V | 7.195 | 7.006 | 6.878 | 6.892 | 6.880 | 6.875 |
| | $^1\Sigma_u^-[F](\pi \to \pi^*)$ | V | 5.628 | 5.360 | 5.273 | 5.281 | 5.270 | 5.260 |
| Cyclopropenone | $^1B_1(n \to \pi^*)$ | V | 4.097 | 4.568 | 4.325 | 4.336 | 4.374 | 4.363 |
| | $^1A_2(n \to \pi^*)$ | V | 5.789 | 5.700 | 5.683 | 5.649 | 5.653 | 5.652 |
| | $^1B_2(n \to 3s)$ | R | 5.962 | 6.480 | 6.391 | 6.383 | 6.425 | 6.416 |
| | $^1B_2(\pi \to \pi^*)$ | V | 6.715 | 6.898 | 6.697 | 6.672 | 6.685 | 6.679 |
| | $^1B_2(n \to 3p)$ | R | 6.454 | 7.039 | 6.919 | 6.906 | 6.952 | 6.941 |
| | $^1A_1(n \to 3p)$ | R | 6.527 | 7.108 | 7.001 | 6.998 | 7.046 | 7.035 |
| | $^1A_1(n.d.)$ | R | 7.889 | 8.370 | 8.281 | 8.271 | 8.288 | 8.284 |
| | $^1A_1(\pi \to \pi^*)$ | V | 8.477 | 8.558 | 8.513 | 8.493 | 8.519 | 8.513 |
| Cyclopropenethione | $^1A_2(n \to \pi^*)$ | V | 3.589 | 3.512 | 3.462 | 3.435 | 3.441 | 3.441 |
| | $^1B_1(n \to \pi^*)$ | V | 3.543 | 3.795 | 3.447 | 3.441 | 3.461 | 3.454 |
| | $^1B_2(\pi \to \pi^*)$ | V | 4.995 | 4.957 | 4.669 | 4.642 | 4.621 | 4.622 |
| | $^1B_2(n \to 3s)$ | R | 5.232 | 5.342 | 5.265 | 5.245 | 5.275 | 5.272 |
| | $^1A_1(\pi \to \pi^*)$ | V | 5.643 | 5.589 | 5.533 | 5.516 | 5.510 | 5.512 |
| | $^1B_2(n \to 3p)$ | R | 5.776 | 5.941 | 5.827 | 5.807 | 5.839 | 5.835 |
| Diacetylene | $^1\Sigma_u^-(\pi \to \pi^*)$ | V | | | | | | |
| | $^1\Delta_u(\pi \to \pi^*)$ | V | | | | | | |
| Glyoxal | $^1A_u(n \to \pi^*)$ | V | 2.976 | 3.033 | 2.939 | 2.938 | 2.937 | 2.938 |
| | $^1B_g(n \to \pi^*)$ | V | 4.518 | 4.441 | 4.344 | 4.320 | 4.314 | 4.315 |
| | $^1A_g(n,n \to \pi^*,\pi^*)$ | V | | | 6.735 | 6.243 | 5.699 | 5.670 |
| | $^1B_g(n \to \pi^*)$ | V | 6.774 | 7.309 | 6.809 | 6.828 | 6.790 | 6.793 |
| | $^1B_u(n \to 3p)$ | R | 7.225 | 7.815 | 7.724 | 7.737 | 7.760 | 7.761 |
| Isobutene | $^1B_1(\pi \to 3s)$ | R | 6.764 | 6.881 | 6.766 | 6.778 | 6.778 | 6.777 |
| | $^1A_1(\pi \to 3p)$ | R | 7.162 | 7.273 | 7.158 | 7.171 | 7.164 | 7.163 |

Follow-up.

| Molecule | State | | CC2 | CCSD | CC3 | CCSDT | CC4 | CCSDTQ |
|---|---|---|---|---|---|---|---|---|
| Methylenecyclopropene | $^1B_2(\pi \to \pi^*)$ | V | 4.633 | 4.620 | 4.381 | 4.365 | 4.341 | 4.343 |
| | $^1B_1(\pi \to 3s)$ | R | 5.647 | 5.740 | 5.651 | 5.659 | 5.660 | 5.658 |
| | $^1A_2(\pi \to 3p)$ | R | 5.948 | 6.064 | 5.972 | 5.981 | 5.983 | 5.981 |
| | $^1A_1(\pi \to \pi^*)$ | V | 6.185 | 6.239 | 6.169 | 6.175 | 6.172 | 6.171 |
| Propynal | $^1A''(n \to \pi^*)$ | V | 4.042 | 3.965 | 3.902 | 3.872 | 3.877 | 3.877 |
| | $^1A''(\pi \to \pi^*)$ | V | 5.887 | 5.899 | 5.695 | 5.729 | 5.700 | 5.700 |
| Thioacetone | $^1A_2(n \to \pi^*)$ | V | 2.682 | 2.631 | 2.582 | 2.556 | 2.561 | 2.560 |
| | $^1B_2(n \to 4s)$ | R | 5.692 | 5.761 | 5.651 | 5.644 | 5.657 | 5.660 |
| | $^1A_1(\pi \to \pi^*)$ | V | 6.302 | 6.207 | 6.091 | 6.100 | 6.064 | 6.066 |
| | $^1B_2(n \to 4p)$ | R | 6.659 | 6.661 | 6.594 | 6.588 | 6.595 | 6.596 |
| | $^1A_1(n \to 4p)$ | R | 6.986 | 7.077 | 6.949 | 6.947 | 6.956 | 6.960 |
| Thioacrolein | $^1A''(n \to \pi^*)$ | V | 2.172 | 2.269 | 2.172 | 2.141 | 2.137 | 2.136 |
| Thiopropynal | $^1A''(n \to \pi^*)$ | V | 2.253 | 2.160 | 2.089 | 2.062 | 2.059 | 2.058 |

Table S8: Vertical transition energies obtained with *aug*-cc-pVDZ for all systems containing four non-hydrogen atoms. See Table S1 for more details.

| Molecule | State | | CC2 | CCSD | CC3 | CCSDT | CC4 | CCSDTQ |
|---|---|---|---|---|---|---|---|---|
| Acetone | $^1A_2(n \rightarrow \pi^*)$ | V | 4.570 | 4.530 | 4.502 | 4.475 | 4.487 | |
| | $^1B_2(n \rightarrow 3s)$ | R | 5.747 | 6.395 | 6.306 | 6.302 | 6.365 | |
| | $^1A_2(n \rightarrow 3p)$ | R | 6.726 | 7.425 | 7.370 | 7.363 | 7.431 | |
| | $^1A_1(n \rightarrow 3p)$ | R | 6.753 | 7.460 | 7.388 | 7.383 | 7.447 | |
| | $^1B_2(n \rightarrow 3p)$ | R | 6.959 | 7.594 | 7.560 | 7.550 | 7.612 | |
| Acrolein | $^1A''(n \rightarrow \pi^*)$ | V | 3.873 | 3.906 | 3.769 | 3.744 | 3.743 | |
| | $^1A'(\pi \rightarrow \pi^*)$ | V | 6.834 | 6.862 | 6.672 | 6.699 | 6.683 | |
| | $^1A''(n \rightarrow \pi^*)$ | V | 6.654 | 7.200 | 6.754 | 6.717 | 6.674 | |
| | $^1A'(n \rightarrow 3s)$ | R | 6.263 | 7.109 | 6.986 | 6.996 | 7.030 | |
| Butadiene | $^1B_u(\pi \rightarrow \pi^*)$ | V | 6.168 | 6.370 | 6.252 | 6.268 | 6.254 | |
| | $^1B_g(\pi \rightarrow 3s)$ | R | 6.131 | 6.302 | 6.258 | 6.270 | 6.277 | |
| | $^1A_g(\pi \rightarrow \pi^*)$ | V | 7.078 | 7.086 | 6.678 | 6.589 | 6.511 | |
| | $^1A_u(\pi \rightarrow 3p)$ | R | 6.450 | 6.619 | 6.574 | 6.588 | 6.594 | |
| | $^1A_u(\pi \rightarrow 3p)$ | R | 6.580 | 6.780 | 6.732 | 6.744 | 6.751 | |
| | $^1B_u(\pi \rightarrow 3p)$ | R | 7.797 | 7.932 | 7.862 | 7.872 | 7.871 | |
| Carbonylfluoride | $^1A_2(n \rightarrow \pi^*)$ | V | 7.501 | 7.359 | 7.341 | 7.309 | 7.321 | 7.321 |
| Cyanoacetylene | $^1\Sigma^-(\pi \rightarrow \pi^*)$ | V | 6.100 | 5.999 | 5.917 | 5.923 | 5.912 | 5.908 |
| | $^1\Delta(\pi \rightarrow \pi^*)$ | V | 6.359 | 6.252 | 6.173 | 6.185 | 6.177 | 6.174 |
| | $^1A''[F](\pi \rightarrow \pi^*)$ | V | 3.805 | 3.653 | 3.605 | 3.623 | 3.633 | |
| Cyanoformaldehyde | $^1A''(n \rightarrow \pi^*)$ | V | 3.994 | 3.939 | 3.864 | 3.841 | 3.843 | |
| | $^1A''(\pi \rightarrow \pi^*)$ | V | 6.810 | 6.765 | 6.510 | 6.544 | 6.514 | |
| Cyanogen | $^1\Sigma_u^-(\pi \rightarrow \pi^*)$ | V | 6.804 | 6.634 | 6.520 | 6.528 | 6.517 | 6.512 |
| | $^1\Delta_u(\pi \rightarrow \pi^*)$ | V | 7.094 | 6.894 | 6.773 | 6.785 | 6.773 | 6.768 |
| | $^1\Sigma_u^-[F](\pi \rightarrow \pi^*)$ | V | 5.555 | 5.276 | 5.194 | 5.200 | 5.189 | 5.180 |
| Cyclopropenone | $^1B_1(n \rightarrow \pi^*)$ | V | 3.986 | 4.472 | 4.217 | 4.233 | 4.270 | |
| | $^1A_2(n \rightarrow \pi^*)$ | V | 5.671 | 5.622 | 5.590 | 5.560 | 5.566 | |
| | $^1B_2(n \rightarrow 3s)$ | R | 5.680 | 6.264 | 6.210 | 6.195 | 6.254 | |
| | $^1B_2(\pi \rightarrow \pi^*)$ | V | 6.564 | 6.785 | 6.558 | 6.539 | 6.550 | |
| | $^1B_2(n \rightarrow 3p)$ | R | 6.366 | 6.957 | 6.879 | 6.862 | 6.920 | |
| | $^1A_1(n \rightarrow 3p)$ | R | 6.310 | 6.944 | 6.878 | 6.865 | 6.929 | |
| | $^1A_1(n.d.)$ | R | 7.554 | 8.126 | 8.086 | 8.069 | 8.116 | |
| | $^1A_1(\pi \rightarrow \pi^*)$ | V | 8.315 | 8.356 | 8.312 | 8.288 | 8.302 | |
| Cyclopropenethione | $^1A_2(n \rightarrow \pi^*)$ | V | 3.592 | 3.542 | 3.474 | 3.450 | 3.453 | |
| | $^1B_1(n \rightarrow \pi^*)$ | V | 3.494 | 3.778 | 3.418 | 3.422 | 3.429 | |
| | $^1B_2(\pi \rightarrow \pi^*)$ | V | 4.937 | 4.955 | 4.658 | 4.638 | 4.613 | |
| | $^1B_2(n \rightarrow 3s)$ | R | 5.100 | 5.276 | 5.227 | 5.205 | 5.244 | |
| | $^1A_1(\pi \rightarrow \pi^*)$ | V | 5.579 | 5.571 | 5.520 | 5.503 | 5.499 | |
| | $^1B_2(n \rightarrow 3p)$ | R | 5.752 | 5.937 | 5.860 | 5.840 | 5.876 | |
| Diacetylene | $^1\Sigma_u^-(\pi \rightarrow \pi^*)$ | V | 5.569 | 5.512 | 5.441 | 5.447 | 5.437 | 5.434 |
| | $^1\Delta_u(\pi \rightarrow \pi^*)$ | V | 5.801 | 5.752 | 5.689 | 5.703 | 5.698 | 5.695 |
| Glyoxal | $^1A_u(n \rightarrow \pi^*)$ | V | 2.929 | 3.010 | 2.899 | 2.900 | 2.898 | |
| | $^1B_g(n \rightarrow \pi^*)$ | V | 4.462 | 4.421 | 4.300 | 4.279 | 4.271 | |
| | $^1A_g(n,n \rightarrow \pi^*,\pi^*)$ | V | | | 6.706 | 6.222 | 5.593 | |
| | $^1B_g(n \rightarrow \pi^*)$ | V | 6.516 | 7.068 | 6.588 | 6.613 | 6.576 | |
| | $^1B_u(n \rightarrow 3p)$ | R | 7.000 | 7.644 | 7.548 | 7.561 | 7.591 | |
| Isobutene | $^1B_1(\pi \rightarrow 3s)$ | R | 6.253 | 6.437 | 6.388 | 6.391 | 6.408 | |
| | $^1A_1(\pi \rightarrow 3p)$ | R | 6.910 | 7.061 | 6.996 | 7.003 | 7.008 | |

Follow-up.

| Molecule | State | | CC2 | CCSD | CC3 | CCSDT | CC4 | CCSDTQ |
|---|---|---|---|---|---|---|---|---|
| Methylenecyclopropene | $^1B_2(\pi \to \pi^*)$ | V | 4.510 | 4.553 | 4.321 | 4.308 | 4.285 | |
| | $^1B_1(\pi \to 3s)$ | R | 5.223 | 5.368 | 5.353 | 5.352 | 5.369 | |
| | $^1A_2(\pi \to 3p)$ | R | 5.727 | 5.895 | 5.876 | 5.875 | 5.893 | |
| | $^1A_1(\pi \to \pi^*)$ | V | 6.101 | 6.178 | 6.150 | 6.149 | 6.157 | |
| Propynal | $^1A''(n \to \pi^*)$ | V | 3.970 | 3.933 | 3.846 | 3.821 | 3.825 | |
| | $^1A''(\pi \to \pi^*)$ | V | 5.772 | 5.773 | 5.587 | 5.617 | 5.591 | |
| Thioacetone | $^1A_2(n \to \pi^*)$ | V | 2.679 | 2.655 | 2.591 | 2.568 | 2.570 | |
| | $^1B_2(n \to 4s)$ | R | 5.374 | 5.529 | 5.441 | 5.433 | 5.457 | |
| | $^1A_1(\pi \to \pi^*)$ | V | 6.136 | 6.068 | 5.968 | 5.978 | 5.947 | |
| | $^1B_2(n \to 4p)$ | R | 6.376 | 6.501 | 6.447 | 6.441 | 6.462 | |
| | $^1A_1(n \to 4p)$ | R | 6.468 | 6.612 | 6.536 | 6.533 | 6.552 | |
| Thioacrolein | $^1A''(n \to \pi^*)$ | V | 2.328 | 2.289 | 2.174 | 2.147 | 2.138 | |
| Thiopropynal | $^1A''(n \to \pi^*)$ | V | 2.240 | 2.175 | 2.089 | 2.063 | 2.058 | |

Table S9: Vertical transition energies obtained with *aug*-cc-pVTZ for all systems containing four non-hydrogen atoms. See Table S1 for more details.

| Molecule | State | | CC2 | CCSD | CC3 | CCSDT | CC4 |
|---|---|---|---|---|---|---|---|
| Acetone | $^1A_2(n \rightarrow \pi^*)$ | V | 4.553 | 4.538 | 4.481 | 4.456 | |
| | $^1B_2(n \rightarrow 3s)$ | R | 5.912 | 6.586 | 6.427 | 6.422 | |
| | $^1A_2(n \rightarrow 3p)$ | R | 6.842 | 7.567 | 7.448 | 7.439 | |
| | $^1A_1(n \rightarrow 3p)$ | R | 6.887 | 7.626 | 7.484 | 7.478 | |
| | $^1B_2(n \rightarrow 3p)$ | R | 7.024 | 7.701 | 7.595 | 7.584 | |
| Acrolein | $^1A''(n \rightarrow \pi^*)$ | V | 3.853 | 3.913 | 3.743 | 3.725 | |
| | $^1A'(\pi \rightarrow \pi^*)$ | V | 6.801 | 6.872 | 6.653 | 6.686 | |
| | $^1A''(n \rightarrow \pi^*)$ | V | 6.681 | 7.269 | 6.752 | 6.730 | |
| | $^1A'(n \rightarrow 3s)$ | R | 6.402 | 7.238 | 7.067 | 7.077 | |
| Butadiene | $^1B_u(\pi \rightarrow \pi^*)$ | V | 6.156 | 6.347 | 6.219 | 6.238 | |
| | $^1B_g(\pi \rightarrow 3s)$ | R | 6.256 | 6.398 | 6.330 | 6.344 | |
| | $^1A_g(\pi \rightarrow \pi^*)$ | V | 7.093 | 7.123 | 6.671 | 6.598 | |
| | $^1A_u(\pi \rightarrow 3p)$ | R | 6.572 | 6.713 | 6.643 | 6.658 | |
| | $^1A_u(\pi \rightarrow 3p)$ | R | 6.702 | 6.874 | 6.799 | 6.814 | |
| | $^1B_u(\pi \rightarrow 3p)$ | R | 7.628 | 7.760 | 7.675 | 7.690 | |
| Carbonylfluoride | $^1A_2(n \rightarrow \pi^*)$ | V | 7.466 | 7.356 | 7.306 | 7.278 | |
| Cyanoacetylene | $^1\Sigma^-(\pi \rightarrow \pi^*)$ | V | 6.031 | 5.882 | 5.803 | 5.809 | 5.792 |
| | $^1\Delta(\pi \rightarrow \pi^*)$ | V | 6.299 | 6.153 | 6.076 | 6.089 | 6.074 |
| | $^1A''[F](\pi \rightarrow \pi^*)$ | V | 3.791 | 3.578 | 3.543 | 3.558 | |
| Cyanoformaldehyde | $^1A''(n \rightarrow \pi^*)$ | V | 3.972 | 3.937 | 3.833 | 3.815 | |
| | $^1A''(\pi \rightarrow \pi^*)$ | V | 6.743 | 6.674 | 6.419 | 6.459 | |
| Cyanogen | $^1\Sigma_u^-(\pi \rightarrow \pi^*)$ | V | 6.721 | 6.497 | 6.389 | 6.399 | 6.380 |
| | $^1\Delta_u(\pi \rightarrow \pi^*)$ | V | 7.017 | 6.776 | 6.659 | 6.673 | 6.654 |
| | $^1\Sigma_u^-[F](\pi \rightarrow \pi^*)$ | V | 5.477 | 5.128 | 5.063 | 5.067 | 5.050 |
| Cyclopropenone | $^1B_1(n \rightarrow \pi^*)$ | V | 4.005 | 4.529 | 4.214 | 4.237 | |
| | $^1A_2(n \rightarrow \pi^*)$ | V | 5.653 | 5.633 | 5.573 | 5.546 | |
| | $^1B_2(n \rightarrow 3s)$ | R | 5.843 | 6.441 | 6.324 | 6.311 | |
| | $^1B_2(\pi \rightarrow \pi^*)$ | V | 6.564 | 6.823 | 6.541 | 6.530 | |
| | $^1B_2(n \rightarrow 3p)$ | R | 6.463 | 7.091 | 6.961 | 6.947 | |
| | $^1A_1(n \rightarrow 3p)$ | R | 6.468 | 7.123 | 6.999 | 6.989 | |
| | $^1A_1(n.d.)$ | R | 7.606 | 8.200 | 8.098 | 8.084 | |
| | $^1A_1(\pi \rightarrow \pi^*)$ | V | 8.280 | 8.352 | 8.284 | 8.262 | |
| Cyclopropenethione | $^1A_2(n \rightarrow \pi^*)$ | V | 3.531 | 3.508 | 3.431 | 3.407 | |
| | $^1B_1(n \rightarrow \pi^*)$ | V | 3.497 | 3.843 | 3.429 | 3.440 | |
| | $^1B_2(\pi \rightarrow \pi^*)$ | V | 4.905 | 4.978 | 4.635 | 4.623 | |
| | $^1B_2(n \rightarrow 3s)$ | R | 5.224 | 5.409 | 5.342 | 5.315 | |
| | $^1A_1(\pi \rightarrow \pi^*)$ | V | 5.585 | 5.554 | 5.491 | 5.473 | |
| | $^1B_2(n \rightarrow 3p)$ | R | 5.819 | 6.031 | 5.926 | 5.904 | |
| Diacetylene | $^1\Sigma_u^-(\pi \rightarrow \pi^*)$ | V | 5.514 | 5.412 | 5.340 | 5.347 | 5.331 |
| | $^1\Delta_u(\pi \rightarrow \pi^*)$ | V | 5.755 | 5.670 | 5.607 | 5.620 | 5.609 |
| Glyoxal | $^1A_u(n \rightarrow \pi^*)$ | V | 2.913 | 3.009 | 2.876 | 2.879 | |
| | $^1B_g(n \rightarrow \pi^*)$ | V | 4.438 | 4.418 | 4.269 | 4.253 | |
| | $^1A_g(n, n \rightarrow \pi^*, \pi^*)$ | V | | | 6.763 | 6.353 | |
| | $^1B_g(n \rightarrow \pi^*)$ | V | 6.511 | 7.123 | 6.578 | 6.614 | |
| | $^1B_u(n \rightarrow 3p)$ | R | 7.161 | 7.836 | 7.673 | 7.690 | |
| Isobutene | $^1B_1(\pi \rightarrow 3s)$ | R | 6.374 | 6.537 | 6.454 | 6.460 | |
| | $^1A_1(\pi \rightarrow 3p)$ | R | 6.952 | 7.086 | 6.996 | 7.006 | |

Follow-up.

| Molecule | State | | CC2 | CCSD | CC3 | CCSDT | CC4 |
|---|---|---|---|---|---|---|---|
| Methylenecyclopropene | $^1B_2(\pi \rightarrow \pi^*)$ | V | 4.507 | 4.583 | 4.313 | 4.306 | |
| | $^1B_1(\pi \rightarrow 3s)$ | R | 5.355 | 5.479 | 5.440 | 5.441 | |
| | $^1A_2(\pi \rightarrow 3p)$ | R | 5.852 | 5.999 | 5.954 | 5.956 | |
| | $^1A_1(\pi \rightarrow \pi^*)$ | V | 6.093 | 6.172 | 6.126 | 6.126 | |
| Propynal | $^1A''(n \rightarrow \pi^*)$ | V | 3.955 | 3.942 | 3.825 | 3.804 | |
| | $^1A''(\pi \rightarrow \pi^*)$ | V | 5.714 | 5.692 | 5.506 | 5.539 | |
| Thioacetone | $^1A_2(n \rightarrow \pi^*)$ | V | 2.630 | 2.628 | 2.553 | 2.528 | |
| | $^1B_2(n \rightarrow 4s)$ | R | 5.502 | 5.672 | 5.555 | 5.542 | |
| | $^1A_1(\pi \rightarrow \pi^*)$ | V | 6.091 | 6.009 | 5.897 | 5.907 | |
| | $^1B_2(n \rightarrow 4p)$ | R | 6.442 | 6.585 | 6.510 | 6.500 | |
| | $^1A_1(n \rightarrow 4p)$ | R | 6.530 | 6.712 | 6.610 | 6.600 | |
| Thioacrolein | $^1A''(n \rightarrow \pi^*)$ | V | 2.281 | 2.264 | 2.139 | 2.113 | |
| Thiopropynal | $^1A''(n \rightarrow \pi^*)$ | V | 2.196 | 2.150 | 2.054 | 2.028 | |

# S2 Transition energies for the largest molecules

Table S10: CC3, CCSDT, and CC4 VTEs (in eV) computed for the five-atom molecules with three atomic basis sets.

| | | CC3 | | | CCSDT | | | CC4 | |
|---|---|---|---|---|---|---|---|---|---|
| Molecule | State | Pop | AVDZ | AVTZ | Pop | AVDZ | AVTZ | Pop | AVDZ |
| Cyclopentadiene | $^1B_2$ (Val, $\pi \to \pi^\star$) | 5.786 | 5.588 | 5.540 | 5.800 | 5.601 | 5.558 | 5.782 | |
| | $^1A_2$ (Ryd, $\pi \to 3s$) | 6.080 | 5.705 | 5.773 | 6.091 | 5.705 | 5.776 | 6.090 | |
| | $^1B_1$ (Ryd, $\pi \to 3p$) | 6.572 | 6.342 | 6.403 | 6.586 | 6.342 | 6.406 | 6.587 | |
| | $^1A_2$ (Ryd, $\pi \to 3p$) | 6.672 | 6.390 | 6.447 | 6.680 | 6.389 | 6.449 | 6.680 | |
| | $^1B_2$ (Ryd, $\pi \to 3p$) | 7.063 | 6.550 | 6.556 | 7.075 | 6.550 | 6.559 | 7.072 | |
| | $^1A_1$ (Val, $\pi \to \pi^\star$) | 6.672 | 6.595 | 6.570 | 6.597 | 6.531 | 6.523 | 6.526 | |
| Difluorodiazirine | $^1B_1$ (Val, $n \to \pi^\star$) | 3.835 | 3.797 | 3.737 | 3.834 | 3.797 | 3.740 | 3.828 | 3.791 |
| | $^1A_2$ (Val, $\pi \to \pi^\star$) | 7.134 | 7.110 | 7.017 | 7.107 | 7.084 | 6.996 | 7.099 | 7.076 |
| | $^1B_2$ (Ryd) | 8.508 | 8.451 | 8.498 | 8.520 | 8.461 | 8.518 | 8.501 | 8.447 |
| Furan | $^1A_2$ (Ryd, $\pi \to 3s$) | 6.264 | 5.999 | 6.078 | 6.277 | 6.003 | 6.087 | 6.272 | 6.013 |
| | $^1B_2$ (Val, $\pi \to \pi^\star$) | 6.499 | 6.370 | 6.343 | 6.522 | 6.391 | 6.370 | 6.496 | 6.367 |
| | $^1A_1$ (Val, $\pi \to \pi^\star$) | 6.707 | 6.616 | 6.584 | 6.672 | 6.584 | 6.563 | 6.636 | 6.551 |
| | $^1B_1$ (Ryd, $\pi \to 3p$) | 6.758 | 6.554 | 6.629 | 6.771 | 6.557 | 6.638 | 6.789 | 6.571 |
| | $^1A_2$ (Ryd, $\pi \to 3p$) | 6.974 | 6.732 | 6.799 | 6.990 | 6.737 | 6.810 | 6.985 | |
| | $^1B_2$ (Ryd, $\pi \to 3p$) | 7.525 | 7.392 | 7.232 | 7.538 | 7.397 | 7.243 | 7.529 | |
| Pyrrole | $^1A_2$ (Ryd, $\pi \to 3s$) | 5.253 | 5.149 | 5.241 | 5.259 | 5.144 | 5.242 | 5.251 | |
| | $^1B_1$ (Ryd) | 5.993 | 5.888 | 5.982 | 5.985 | 5.869 | 5.970 | 5.985 | |
| | $^1A_2$ (Ryd, $\pi \to 3p$) | 6.273 | 5.941 | 6.014 | 6.279 | 5.934 | 6.012 | 6.275 | |
| | $^1B_1$ (Ryd) | 6.169 | 6.013 | 6.099 | 6.173 | 6.002 | 6.092 | 6.172 | |
| | $^1B_2$ (Val, $\pi \to \pi^\star$) | 6.330 | 6.280 | 6.251 | 6.335 | 6.278 | 6.254 | 6.318 | |
| | $^1A_1$ (Val, $\pi \to \pi^\star$) | 6.428 | 6.349 | 6.315 | 6.399 | 6.321 | 6.298 | 6.374 | |
| | $^1B_2$ (Ryd, $\pi \to 3p$) | 7.198 | 7.005 | 6.830 | 7.204 | 7.004 | 6.835 | 7.190 | |
| Thiopehene | $^1A_1$ (Val, $\pi \to \pi^\star$) | 5.789 | 5.697 | 5.650 | 5.766 | 5.766 | 5.635 | 5.751 | |
| | $^1B_2$ (Val, $\pi \to \pi^\star$) | 6.229 | 6.047 | 5.959 | 6.238 | 6.055 | 5.975 | 6.206 | |
| | $^1A_2$ (Ryd, $\pi \to 3s$) | 6.263 | 6.070 | 6.141 | 6.257 | 6.058 | 6.135 | 6.249 | |
| | $^1B_1$ (Ryd, $\pi \to 3p$) | 6.181 | 6.189 | 6.136 | 6.165 | 6.173 | 6.129 | 6.152 | |
| | $^1A_2$ (Ryd, $\pi \to 3p$) | 6.317 | 6.329 | 6.252 | 6.306 | 6.311 | 6.239 | 6.301 | |
| | $^1B_1$ (Ryd, $\pi \to 3s$) | 6.621 | 6.424 | 6.502 | 6.615 | 6.410 | 6.492 | 6.612 | |
| | $^1B_2$ (Ryd, $\pi \to 3p$) | 7.450 | 7.450 | 7.295 | 7.444 | 7.435 | 7.287 | 7.431 | |
| | $^1A_1$ (Val, $\pi \to \pi^\star$) | 7.496 | 7.408 | 7.352 | 7.461 | 7.381 | 7.339 | 7.420 | |

Table S11: CC3, CCSDT, and CC4 VTEs (in eV) computed for the six-atom molecules with three atomic basis sets.

| | | CC3 | | | CCSDT | | | CC4 |
|---|---|---|---|---|---|---|---|---|
| Molecule | State | Pop | AVDZ | AVTZ | Pop | AVDZ | AVTZ | Pop |
| Benzene | $^1B_{2u}$ (Val, $\pi \to \pi^\star$) | 5.134 | 5.114 | 5.086 | 5.102 | 5.083 | 5.062 | 5.085 |
| | $^1B_{1u}$ (Val, $\pi \to \pi^\star$) | 6.682 | 6.498 | 6.442 | 6.691 | 6.502 | 6.447 | 6.677 |
| | $^1E_{1g}$ (Ryd, $\pi \to 3s$) | 6.749 | 6.456 | 6.520 | 6.763 | 6.457 | 6.524 | 6.755 |
| | $^1A_{2u}$ (Ryd, $\pi \to 3p$) | 7.235 | 7.020 | 7.079 | 7.255 | 7.022 | 7.084 | 7.250 |
| | $^1E_{2u}$ (Ryd, $\pi \to 3p$) | 7.335 | 7.087 | 7.147 | 7.353 | 7.089 | 7.151 | 7.348 |
| | $^1A_{1u}$ (Ryd, $\pi \to 3p$) | 7.466 | 7.178 | 7.237 | 7.482 | 7.180 | 7.241 | 7.473 |
| | $^1E_{1u}$ (Val, $\pi \to \pi^\star$) | 7.350 | 7.216 | 7.169 | 7.376 | 7.238 | 7.197 | 7.348 |
| Hexatriene | $^1B_u$ (Val, $\pi \to \pi^\star$) | 5.538 | 5.372 | 5.336 | 5.562 | 5.397 | | 5.543 |
| | $^1A_g$ (Val, $\pi \to \pi^\star$) | 5.759 | 5.755 | 5.747 | 5.617 | 5.627 | | 5.471 |
| | $^1A_u$ (Ryd, $\pi \to 3s$) | 6.036 | 5.710 | 5.781 | 6.078 | 5.728 | | 6.048 |
| | $^1B_g$ (Ryd, $\pi \to 3p$) | 6.052 | 5.843 | 5.917 | 6.061 | 5.862 | | 6.065 |
| Pyrazine | $^1B_{3u}$ (Val, $n \to \pi^\star$) | 4.281 | 4.189 | 4.142 | 4.282 | 4.190 | 4.149 | 4.277 |
| | $^1A_u$ (Val, $n \to \pi^\star$) | 5.078 | 4.976 | 4.967 | 5.078 | 4.978 | 4.977 | 5.071 |
| | $^1B_{2u}$ (Val, $\pi \to \pi^\star$) | 5.101 | 5.070 | 5.029 | 5.082 | 5.053 | 5.018 | 5.052 |
| | $^1B_{2g}$ (Val, $n \to \pi^\star$) | 5.863 | 5.780 | 5.714 | 5.846 | 5.767 | 5.711 | 5.817 |
| | $^1A_g$ (Ryd, $n \to 3s$) | 6.740 | 6.541 | 6.656 | 6.736 | 6.528 | 6.650 | 6.749 |
| | $^1B_{1g}$ (Val, $n \to \pi^\star$) | 6.865 | 6.752 | 6.725 | 6.856 | 6.749 | 6.737 | 6.822 |
| | $^1B_{1u}$ (Val, $\pi \to \pi^\star$) | 7.096 | 6.925 | 6.862 | 7.107 | 6.933 | 6.874 | 7.086 |
| | $^1B_{1g}$ (Ryd, $\pi \to 3s$) | 7.362 | 7.135 | 7.202 | 7.377 | 7.141 | 7.214 | 7.366 |
| | $^1B_{2u}$ (Ryd, $n \to 3p$) | 7.389 | 7.139 | 7.253 | 7.394 | 7.131 | 7.252 | 7.409 |
| | $^1B_{1u}$ (Ryd, $n \to 3p$) | 7.556 | 7.377 | 7.453 | 7.555 | 7.365 | 7.448 | 7.559 |
| | $^1B_{1u}$ (Val, $\pi \to \pi^\star$) | 8.191 | 7.992 | 7.938 | 8.228 | 8.023 | 7.981 | 8.186 |
| Tetrazine | $^1B_{3u}$ (Val, $n \to \pi^\star$) | 2.528 | 2.487 | 2.455 | 2.539 | 2.499 | 2.470 | 2.531 |
| | $^1A_u$ (Val, $n \to \pi^\star$) | 3.746 | 3.689 | 3.674 | 3.752 | 3.699 | 3.692 | 3.739 |
| | $^1A_g$ (Val, $n,n \to \pi^\star\pi^\star$) | 6.222 | 6.218 | 6.209 | 5.856 | 5.858 | 5.958 | 5.063 |
| | $^1B_{1g}$ (Val, $n \to \pi^\star$) | 5.012 | 4.966 | 4.910 | 5.022 | 4.977 | 4.935 | 4.953 |
| | $^1B_{2u}$ (Val, $\pi \to \pi^\star$) | 5.288 | 5.270 | 5.227 | 5.261 | 5.246 | 5.211 | 5.223 |
| | $^1B_{2g}$ (Val, $n \to \pi^\star$) | 5.557 | 5.533 | 5.464 | 5.522 | 5.502 | 5.450 | 5.467 |
| | $^1A_u$ (Val, $n \to \pi^\star$) | 5.608 | 5.589 | 5.524 | 5.611 | 5.593 | 5.534 | 5.590 |
| | $^1B_{3g}$ (Val, $n,n \to \pi^\star\pi^\star$) | 7.640 | 7.618 | 7.617 | 7.300 | 7.302 | 7.434 | 6.308 |
| | $^1B_{2g}$ (Val, $n \to \pi^\star$) | 6.236 | 6.171 | 6.132 | 6.221 | 6.163 | 6.144 | 6.130 |
| | $^1B_{3g}$ (Ryd, $n \to 3s$) | 6.512 | 6.345 | 6.466 | 6.498 | 6.327 | 6.455 | 6.509 |
| | $^1B_{3u}$ (Val, $\pi \to \pi^\star$) | 6.767 | 6.727 | 6.685 | 6.771 | 6.733 | 6.702 | 6.742 |
| | $^1B_{1g}$ (Val, $n \to \pi^\star$) | 7.039 | 6.976 | 6.917 | 7.038 | 6.978 | 6.933 | 6.999 |

# S3 Geometries

Below, we provide the cartesian coordinates of the compounds investigated in this study. These are provided in atomic units (bohr) and have been extracted from the QUEST database.

## S3.1 Acetaldehyde

| | | | |
|---|---|---|---|
| C | -0.00234503 | 0.00000000 | 0.87125063 |
| C | -1.75847785 | 0.00000000 | -1.34973671 |
| O | 2.27947397 | 0.00000000 | 0.71968028 |
| H | -0.92904537 | 0.00000000 | 2.73929404 |
| H | -2.97955463 | 1.66046488 | -1.25209463 |
| H | -2.97955463 | -1.66046488 | -1.25209463 |
| H | -0.70043433 | 0.00000000 | -3.11066412 |

## S3.2 Acetone

| | | | |
|---|---|---|---|
| C | 0.00000000 | 0.00000000 | 0.18807702 |
| C | 0.00000000 | 2.42007545 | -1.31764698 |
| C | 0.00000000 | -2.42007545 | -1.31764698 |
| O | 0.00000000 | 0.00000000 | 2.48269094 |
| H | 0.00000000 | 4.03690733 | -0.05185132 |
| H | 0.00000000 | -4.03690733 | -0.05185132 |
| H | 1.66061256 | 2.48420530 | -2.53995285 |
| H | -1.66061256 | 2.48420530 | -2.53995285 |
| H | 1.66061256 | -2.48420530 | -2.53995285 |
| H | -1.66061256 | -2.48420530 | -2.53995285 |

## S3.3 Acetylene

Ground state

| | | | |
|---|---|---|---|
| C | 0.00000000 | 0.00000000 | 1.14048351 |
| C | 0.00000000 | 0.00000000 | -1.14048351 |
| H | 0.00000000 | 0.00000000 | 3.14009043 |
| H | 0.00000000 | 0.00000000 | -3.14009043 |

*Trans* excited state ($^1A_u$ state in the $C_{2h}$ point group)

| | | | |
|---|---|---|---|
| C | 1.29567779 | 0.00000000 | -0.01846047 |
| C | -1.29567779 | 0.00000000 | 0.01846047 |
| H | 2.41938674 | 0.00000000 | 1.70881682 |
| H | -2.41938674 | 0.00000000 | -1.70881682 |

*Cis* excited state ($^1A_2$ state in the $C_{2v}$ point group)

| | | | |
|---|---|---|---|
| C | 0.00000000 | 1.26834508 | -0.11726146 |
| C | 0.00000000 | -1.26834508 | -0.11726146 |
| H | 0.00000000 | 2.67282325 | 1.39629264 |
| H | 0.00000000 | -2.67282325 | 1.39629264 |

## S3.4 Acrolein

| | | | |
|---|---|---|---|
| C | -1.11645072 | -0.68348783 | 0.00000000 |
| C | 1.20647847 | 0.83714564 | 0.00000000 |
| C | 3.46831059 | -0.28872636 | 0.00000000 |
| O | -3.23666415 | 0.19187203 | 0.00000000 |
| H | -0.80613858 | -2.74747338 | 0.00000000 |
| H | 0.98699813 | 2.86613511 | 0.00000000 |
| H | 5.20930864 | 0.77443560 | 0.00000000 |
| H | 3.60951559 | -2.33000749 | 0.00000000 |

## S3.5 Benzene

| | | | |
|---|---|---|---|
| C | 0.00000000 | 2.63144965 | 0.00000000 |
| C | -2.27890225 | 1.31572483 | 0.00000000 |
| C | -2.27890225 | -1.31572483 | 0.00000000 |
| C | 0.00000000 | -2.63144965 | 0.00000000 |
| C | 2.27890225 | -1.31572483 | 0.00000000 |
| C | 2.27890225 | 1.31572483 | 0.00000000 |
| H | -4.04725813 | 2.33668557 | 0.00000000 |
| H | -4.04725813 | -2.33668557 | 0.00000000 |
| H | -0.00000000 | -4.67337115 | 0.00000000 |
| H | 4.04725813 | -2.33668557 | 0.00000000 |
| H | 4.04725813 | 2.33668557 | 0.00000000 |
| H | 0.00000000 | 4.67337115 | 0.00000000 |

## S3.6 Butadiene

| | | | |
|---|---|---|---|
| C | 1.14656244 | 0.00000000 | 0.75468820 |
| C | -1.14656244 | 0.00000000 | -0.75468820 |
| C | 3.48132647 | 0.00000000 | -0.22482805 |
| C | -3.48132647 | 0.00000000 | 0.22482805 |
| H | 0.90770978 | 0.00000000 | 2.78883925 |
| H | -0.90770978 | 0.00000000 | -2.78883925 |
| H | 3.77525814 | 0.00000000 | -2.24895470 |
| H | -3.77525814 | 0.00000000 | 2.24895470 |
| H | 5.13664967 | 0.00000000 | 0.96861890 |
| H | -5.13664967 | 0.00000000 | -0.96861890 |

## S3.7 Carbonylfluoride

| | | | |
|---|---|---|---|
| C | 0.00000000 | 0.00000000 | -0.30652633 |
| O | 0.00000000 | 0.00000000 | -2.52469534 |
| F | 0.00000000 | 2.00254958 | 1.16003038 |
| F | 0.00000000 | -2.00254958 | 1.16003038 |

## S3.8 $CCl_2$

| | | | |
|---|---|---|---|
| C | 0.00000000 | 0.00000000 | -1.60920674 |
| Cl | 0.00000000 | 2.65360612 | 0.27602958 |
| Cl | 0.00000000 | -2.65360612 | 0.27602958 |

## S3.9 CClF

| | | | |
|---|---|---|---|
| C | 0.29776085 | 0.00000000 | 1.47969075 |
| F | 2.16980264 | 0.00000000 | -0.10569879 |
| Cl | -2.46756349 | 0.00000000 | -0.32822320 |

## S3.10 $CF_2$

| | | | |
|---|---|---|---|
| C | 0.00000000 | 0.00000000 | -1.14170749 |
| F | 0.00000000 | 1.94810617 | 0.36114458 |
| F | 0.00000000 | -1.94810617 | 0.36114458 |

## S3.11 Cyanoacetylene

| | | | |
|---|---|---|---|
| C | 0.00000000 | 0.00000000 | -3.59120182 |
| C | 0.00000000 | 0.00000000 | -1.30693904 |
| C | 0.00000000 | 0.00000000 | 1.28880240 |
| N | 0.00000000 | 0.00000000 | 3.48692211 |
| H | 0.00000000 | 0.00000000 | -5.59619886 |

Lowest excited state

| | | | |
|---|---|---|---|
| C | 1.99411175 | 0.00000000 | 2.81781077 |
| C | -0.07304269 | 0.00000000 | 1.33125774 |
| C | -0.63630126 | 0.00000000 | -1.14556678 |
| N | -1.39755756 | 0.00000000 | -3.26154643 |
| H | 1.90749857 | 0.00000000 | 4.87279180 |

## S3.12 Cyanoformaldehyde

| | | | |
|---|---|---|---|
| C | -0.91561483 | 0.00000000 | -1.22522833 |
| C | -0.01092219 | 0.00000000 | 1.39523175 |
| N | 0.64170259 | 0.00000000 | 3.48820325 |
| O | 0.50833684 | 0.00000000 | -3.00337867 |
| H | -2.97202213 | 0.00000000 | -1.42565674 |

## S3.13 Cyanogen

Ground state

| | | | |
|---|---|---|---|
| C | 0.00000000 | 0.00000000 | 1.30401924 |
| C | 0.00000000 | 0.00000000 | -1.30401924 |
| N | 0.00000000 | 0.00000000 | 3.49784121 |
| N | 0.00000000 | 0.00000000 | -3.49784121 |

Lowest excited state

| | | | |
|---|---|---|---|
| C | 0.00000000 | 0.00000000 | 1.22784115 |
| C | 0.00000000 | 0.00000000 | -1.22784115 |
| N | 0.00000000 | 0.00000000 | 3.56462559 |
| N | 0.00000000 | 0.00000000 | -3.56462559 |

## S3.14 Cyclopentadiene

| | | | |
|---|---|---|---|
| C | 0.00000000 | 0.00000000 | -2.33113051 |
| C | 0.00000000 | 2.22209092 | -0.56871188 |
| C | 0.00000000 | -2.22209092 | -0.56871188 |
| C | 0.00000000 | 1.38514451 | 1.83772922 |
| C | 0.00000000 | -1.38514451 | 1.83772922 |
| H | 1.66130504 | 0.00000000 | -3.56414299 |
| H | -1.66130504 | 0.00000000 | -3.56414299 |
| H | 0.00000000 | 4.16550405 | -1.18116624 |
| H | 0.00000000 | -4.16550405 | -1.18116624 |
| H | 0.00000000 | 2.54514584 | 3.51352303 |
| H | 0.00000000 | -2.54514584 | 3.51352303 |

## S3.15 Cyclopropene

| | | | |
|---|---|---|---|
| C | 0.00000000 | 0.00000000 | -1.66820880 |
| C | 0.00000000 | 1.22523906 | 0.90681419 |
| C | 0.00000000 | -1.22523906 | 0.90681419 |
| H | 1.72255446 | 0.00000000 | -2.77881149 |
| H | -1.72255446 | 0.00000000 | -2.77881149 |
| H | 0.00000000 | 2.97844519 | 1.92076771 |
| H | 0.00000000 | -2.97844519 | 1.92076771 |

## S3.16 Cyclopropenone

| | | | |
|---|---|---|---|
| C | 0.00000000 | 1.27491826 | -1.86930519 |
| C | 0.00000000 | -1.27491826 | -1.86930519 |
| C | 0.00000000 | 0.00000000 | 0.51814554 |
| O | 0.00000000 | 0.00000000 | 2.79326776 |
| H | 0.00000000 | 2.92791371 | -3.05679837 |
| H | 0.00000000 | -2.92791371 | -3.05679837 |

## S3.17 Cyclopropenethione

| | | | |
|---|---|---|---|
| C | 0.00000000 | 1.26230744 | -2.86571925 |
| C | 0.00000000 | -1.26230744 | -2.86571925 |
| C | 0.00000000 | 0.00000000 | -0.49233236 |
| S | 0.00000000 | 0.00000000 | 2.57821680 |
| H | 0.00000000 | 2.97773331 | -3.95114059 |
| H | 0.00000000 | -2.97773331 | -3.95114059 |

## S3.18 Diacetylene

| | | | |
|---|---|---|---|
| C | 0.00000000 | 0.00000000 | 1.29447700 |
| C | 0.00000000 | 0.00000000 | -1.29447700 |
| C | 0.00000000 | 0.00000000 | 3.58448429 |
| C | 0.00000000 | 0.00000000 | -3.58448429 |
| H | 0.00000000 | 0.00000000 | 5.58943003 |
| H | 0.00000000 | 0.00000000 | -5.58943003 |

## S3.19 Diazirine

| | | | |
|---|---|---|---|
| C | 0.00000000 | 0.00000000 | -0.26696099 |
| H | 0.00000000 | 1.75890895 | -1.28616478 |
| H | 0.00000000 | -1.75890895 | -1.28616478 |
| N | 1.16058100 | 0.00000000 | 2.27183007 |
| N | -1.16058100 | 0.00000000 | 2.27183007 |

## S3.20 Diazomethane

Ground state

| | | | |
|---|---|---|---|
| C | 0.00000000 | 0.00000000 | -2.30830005 |
| N | 0.00000000 | 0.00000000 | 0.14457890 |
| N | 0.00000000 | 0.00000000 | 2.29923216 |
| H | 0.00000000 | 1.79875201 | -3.24272317 |
| H | 0.00000000 | -1.79875201 | -3.24272317 |

Excited state ($^1A$" state in the $C_s$ point group)

| | | | |
|---|---|---|---|
| C | 1.80206107 | 0.00000000 | -1.03389466 |
| N | -0.01743713 | 0.00000000 | 0.84742344 |
| N | -2.25203764 | 0.00000000 | 0.54034983 |
| H | 3.74280590 | 0.00000000 | -0.44375913 |
| H | 1.20115546 | 0.00000000 | -2.98380249 |

## S3.21 Difluorodiazirine ($CF_2N_2$)

| | | | |
|---|---|---|---|
| C | 0.00000000 | 0.00000000 | -0.15283028 |
| F | 0.00000000 | 2.06077297 | -1.57706828 |
| F | 0.00000000 | -2.06077297 | -1.57706828 |
| N | 1.20382241 | 0.00000000 | 2.20566821 |
| N | -1.20382241 | 0.00000000 | 2.20566821 |

## S3.22 Ethylene

| | | | |
|---|---|---|---|
| C | 0.00000000 | 1.26026583 | 0.00000000 |
| C | 0.00000000 | -1.26026583 | 0.00000000 |
| H | 0.00000000 | 2.32345976 | 1.74287672 |
| H | 0.00000000 | -2.32345976 | 1.74287672 |
| H | 0.00000000 | 2.32345976 | -1.74287672 |
| H | 0.00000000 | -2.32345976 | -1.74287672 |

## S3.23 Formaldehyde

Ground state

| | | | |
|---|---|---|---|
| C | 0.00000000 | 0.00000000 | -1.13947666 |
| O | 0.00000000 | 0.00000000 | 1.14402883 |
| H | 0.00000000 | 1.76627623 | -2.23398653 |
| H | 0.00000000 | -1.76627623 | -2.23398653 |

Excited state ($^1A$" state in the $C_s$ point group)

| | | | |
|---|---|---|---|
| C | -0.09942705 | 0.00000000 | 1.27071070 |
| O | 0.01987299 | 0.00000000 | -1.23280536 |
| H | 0.42778855 | 1.76729629 | 2.18470884 |
| H | 0.42778855 | -1.76729629 | 2.18470884 |

## S3.24 Formamide

| | | | |
|---|---|---|---|
| C | 0.00183118 | 0.00000000 | 0.79313299 |
| O | 2.26817156 | 0.00000000 | 0.43918824 |
| N | -1.76886033 | 0.00000000 | -1.06219243 |
| H | -0.84133459 | 0.00000000 | 2.68872485 |
| H | -1.21254414 | 0.00000000 | -2.87596907 |
| H | -3.61627502 | 0.00000000 | -0.65031317 |

## S3.25 Formylfluoride

| | | | |
|---|---|---|---|
| C | 0.00536098 | 0.00000000 | 0.75320959 |
| O | 2.17369813 | 0.00000000 | 0.22287752 |
| H | -0.83846350 | 0.00000000 | 2.62640974 |
| F | -1.84051320 | 0.00000000 | -0.99373750 |

## S3.26 Furan

| | | | |
|---|---|---|---|
| C | 0.00000000 | 2.06365826 | -0.60051250 |
| C | 0.00000000 | -2.06365826 | -0.60051250 |
| C | 0.00000000 | 1.35348578 | 1.86336416 |
| C | 0.00000000 | -1.35348578 | 1.86336416 |
| O | 0.00000000 | 0.00000000 | -2.13945332 |
| H | 0.00000000 | 3.86337287 | -1.53765695 |
| H | 0.00000000 | -3.86337287 | -1.53765695 |
| H | 0.00000000 | 2.59168789 | 3.47168051 |
| H | 0.00000000 | -2.59168789 | 3.47168051 |

## S3.27 Glyoxal

| | | | |
|---|---|---|---|
| C | 1.21360282 | 0.75840215 | 0.00000000 |
| C | -1.21360282 | -0.75840215 | 0.00000000 |
| O | 3.25581408 | -0.26453186 | 0.00000000 |
| O | -3.25581408 | 0.26453186 | 0.00000000 |
| H | 0.96135276 | 2.81883243 | 0.00000000 |
| H | -0.96135276 | -2.81883243 | 0.00000000 |

## S3.28 HCCl

| | | | |
|---|---|---|---|
| H | -1.88068369 | 0.00000000 | -0.14323924 |
| Cl | 2.28559426 | 0.00000000 | -0.43261163 |
| C | -0.40491057 | 0.00000000 | 1.32161964 |

## S3.29 HCF

| | | | |
|---|---|---|---|
| C | -0.13561085 | 0.00000000 | 1.20394474 |
| F | 1.85493976 | 0.00000000 | -0.27610752 |
| H | -1.71932891 | 0.00000000 | -0.18206846 |

## S3.30 HCP

| | | | |
|---|---|---|---|
| H | 0.00000000 | 0.00000000 | -4.03090449 |
| C | 0.00000000 | 0.00000000 | -2.01691641 |
| P | 0.00000000 | 0.00000000 | 0.91401621 |

## S3.31 Hexatriene

| | | | |
|---|---|---|---|
| C | 1.14024826 | 0.56596845 | 0.00000000 |
| C | -1.14024826 | -0.56596845 | 0.00000000 |
| C | 3.51540649 | -0.78907931 | 0.00000000 |
| C | -3.51540649 | 0.78907931 | 0.00000000 |
| C | 5.78668151 | 0.33754155 | 0.00000000 |
| C | -5.78668151 | -0.33754155 | 0.00000000 |
| H | 1.23448067 | 2.61584039 | 0.00000000 |
| H | -1.23448067 | -2.61584039 | 0.00000000 |
| H | 3.40773630 | -2.83459321 | 0.00000000 |
| H | -3.40773630 | 2.83459321 | 0.00000000 |
| H | 5.95047109 | 2.37626316 | 0.00000000 |
| H | -5.95047109 | -2.37626316 | 0.00000000 |
| H | 7.51470672 | -0.74809921 | 0.00000000 |
| H | -7.51470672 | 0.74809921 | 0.00000000 |

## S3.32 HPO

| | | | |
|---|---|---|---|
| H | 0.31668637 | 0.00000000 | 0.14072725 |
| P | -0.80573521 | 0.00000000 | 2.65136926 |
| O | 1.43391190 | 0.00000000 | 4.38886277 |

## S3.33 HPS

| | | | |
|---|---|---|---|
| H | -2.56278959 | 0.00000000 | 2.36296006 |
| P | 0.09114182 | 0.00000000 | 1.82568543 |
| S | 0.07946992 | 0.00000000 | -1.85778170 |

## S3.34 HSiF

| | | | |
|---|---|---|---|
| Si | -0.06438136 | 0.00000000 | 1.67253150 |
| F | 2.24990164 | 0.00000000 | -0.33928119 |
| H | -2.18552027 | 0.00000000 | -0.28748154 |

## S3.35 Isobutene

| | | | |
|---|---|---|---|
| C | 0.00000000 | 0.00000000 | 2.70790758 |
| C | 0.00000000 | 0.00000000 | 0.18431282 |
| C | 0.00000000 | 2.39894572 | -1.32482735 |
| C | 0.00000000 | -2.39894572 | -1.32482735 |
| H | 0.00000000 | 1.74848405 | 3.76691310 |
| H | 0.00000000 | -1.74848405 | 3.76691310 |
| H | 0.00000000 | 4.05897160 | -0.10582007 |
| H | 0.00000000 | -4.05897160 | -0.10582007 |
| H | 1.66026992 | 2.48337908 | -2.55086178 |
| H | -1.66026992 | 2.48337908 | -2.55086178 |
| H | 1.66026992 | -2.48337908 | -2.55086178 |
| H | -1.66026992 | -2.48337908 | -2.55086178 |

## S3.36 Ketene

Ground state

| | | | |
|---|---|---|---|
| C | 0.00000000 | 0.00000000 | -2.44810151 |
| C | 0.00000000 | 0.00000000 | 0.03498545 |
| O | 0.00000000 | 0.00000000 | 2.23663914 |
| H | 0.00000000 | 1.77432079 | -3.43705988 |
| H | 0.00000000 | -1.77432079 | -3.43705988 |

Excited state ($^1A$" state in the $C_s$ point group)

| | | | |
|---|---|---|---|
| C | 2.04306304 | 0.00000000 | -0.93056721 |
| C | 0.00400918 | 0.00000000 | 0.83531393 |
| O | -2.23710378 | 0.00000000 | 0.46984584 |
| H | 1.63603518 | 0.00000000 | -2.93687368 |
| H | 3.96212800 | 0.00000000 | -0.26649149 |

## S3.37 Methanimine

| | | | |
|---|---|---|---|
| C | 0.10696646 | 0.00000000 | 1.11091130 |
| N | 0.10764012 | 0.00000000 | -1.29677742 |
| H | -1.59140953 | 0.00000000 | 2.27296652 |
| H | 1.90475160 | 0.00000000 | 2.09393982 |
| H | -1.69956184 | 0.00000000 | -1.96217482 |

## S3.38 Methylenecyclopropene

| | | | |
|---|---|---|---|
| C | 0.00000000 | 0.00000000 | 0.53512883 |
| C | 0.00000000 | 0.00000000 | 3.04739824 |
| C | 0.00000000 | 1.25042956 | -1.88571561 |
| C | 0.00000000 | -1.25042956 | -1.88571561 |
| H | 0.00000000 | 2.96887531 | -2.96270271 |
| H | 0.00000000 | -2.96887531 | -2.96270271 |
| H | 0.00000000 | 1.75335023 | 4.08608382 |
| H | 0.00000000 | -1.75335023 | 4.08608382 |

## S3.39 Nitrosomethane

Ground state

| | | | |
|---|---|---|---|
| C | -1.78426612 | 0.00000000 | -1.07224050 |
| N | -0.00541753 | 0.00000000 | 1.08060391 |
| O | 2.18814985 | 0.00000000 | 0.43452135 |
| H | -0.77343975 | 0.00000000 | -2.86415606 |
| H | -2.97471478 | 1.66801808 | -0.86424584 |
| H | -2.97471478 | -1.66801808 | -0.86424584 |

Excited state ($^1A$" state in the $C_s$ point group)

| | | | |
|---|---|---|---|
| C | 1.86306273 | 0.00000000 | -1.06035094 |
| N | 0.00638693 | 0.00000000 | 1.02546010 |
| O | -2.26923072 | 0.00000000 | 0.47699489 |
| H | 3.72600129 | 0.00000000 | -0.21094854 |
| H | 1.58491147 | 1.68964774 | -2.20977225 |
| H | 1.58491147 | -1.68964774 | -2.20977225 |

## S3.40 Nitroxyl

| | | | |
|---|---|---|---|
| O | 0.21099695 | 0.00000000 | 2.15462460 |
| N | -0.44776863 | 0.00000000 | -0.03589263 |
| H | 1.18163475 | 0.00000000 | -1.17386890 |

## S3.41 Propynal

| | | | |
|---|---|---|---|
| C | -0.78051115 | 0.00000000 | -1.38900384 |
| C | -0.17873562 | 0.00000000 | 1.27825868 |
| C | 0.23763714 | 0.00000000 | 3.52644798 |
| O | 0.80143996 | 0.00000000 | -3.04628328 |
| H | -2.80713069 | 0.00000000 | -1.82768750 |
| H | 0.64026209 | 0.00000000 | 5.48853193 |

## S3.42 Pyrazine

| | | | |
|---|---|---|---|
| C | 0.00000000 | 2.13188686 | 1.31510863 |
| C | 0.00000000 | -2.13188686 | 1.31510863 |
| C | 0.00000000 | 2.13188686 | -1.31510863 |
| C | 0.00000000 | -2.13188686 | -1.31510863 |
| N | 0.00000000 | 0.00000000 | 2.66620111 |
| N | 0.00000000 | 0.00000000 | -2.66620111 |
| H | 0.00000000 | 3.88751412 | 2.35234226 |
| H | 0.00000000 | -3.88751412 | 2.35234226 |
| H | 0.00000000 | 3.88751412 | -2.35234226 |
| H | 0.00000000 | -3.88751412 | -2.35234226 |

## S3.43 Pyrrole

| | | | |
|---|---|---|---|
| C | 0.00000000 | 2.11924634 | 0.62676569 |
| C | 0.00000000 | -2.11924634 | 0.62676569 |
| C | 0.00000000 | 1.34568862 | -1.85506908 |
| C | 0.00000000 | -1.34568862 | -1.85506908 |
| N | 0.00000000 | 0.00000000 | 2.10934391 |
| H | 0.00000000 | 0.00000000 | 4.00257355 |
| H | 0.00000000 | 3.97648410 | 1.44830201 |
| H | 0.00000000 | -3.97648410 | 1.44830201 |
| H | 0.00000000 | 2.56726559 | -3.47837232 |
| H | 0.00000000 | -2.56726559 | -3.47837232 |

## S3.44 $SiCl_2$

| | | | |
|---|---|---|---|
| Si | 0.00000000 | 0.00000000 | -1.78528322 |
| Cl | 0.00000000 | 3.04414528 | 0.71619419 |
| Cl | 0.00000000 | -3.04414528 | 0.71619419 |

## S3.45 Silylidene

| | | | |
|---|---|---|---|
| C | 0.00000000 | 0.00000000 | -2.09539928 |
| Si | 0.00000000 | 0.00000000 | 1.14992930 |
| H | 0.00000000 | 1.70929524 | -3.22894481 |
| H | 0.00000000 | -1.70929524 | -3.22894481 |

## S3.46 Streptocyanine-C1

| | | | |
|---|---|---|---|
| C | 0.00000000 | 0.00000000 | 0.80488833 |
| N | 0.00000000 | 2.19423463 | -0.33580561 |
| N | 0.00000000 | -2.19423463 | -0.33580561 |
| H | 0.00000000 | 0.00000000 | 2.84436959 |
| H | 0.00000000 | 2.36978315 | -2.23371976 |
| H | 0.00000000 | -2.36978315 | -2.23371976 |
| H | 0.00000000 | 3.79412648 | 0.69399206 |
| H | 0.00000000 | -3.79412648 | 0.69399206 |

## S3.47 Tetrazine

| | | | |
|---|---|---|---|
| C | 0.00000000 | 0.00000000 | 2.38208164 |
| C | 0.00000000 | 0.00000000 | -2.38208164 |
| N | 2.25673244 | 0.00000000 | 1.24973261 |
| N | -2.25673244 | 0.00000000 | 1.24973261 |
| N | 2.25673244 | 0.00000000 | -1.24973261 |
| N | -2.25673244 | 0.00000000 | -1.24973261 |
| H | 0.00000000 | 0.00000000 | 4.41850901 |
| H | 0.00000000 | 0.00000000 | -4.41850901 |

## S3.48 Thioacetone

| | | | |
|---|---|---|---|
| C | 0.00000000 | 0.00000000 | 0.68476030 |
| C | 0.00000000 | 2.38541696 | 2.20685096 |
| C | 0.00000000 | -2.38541696 | 2.20685096 |
| S | 0.00000000 | 0.00000000 | -2.39920303 |
| H | 0.00000000 | 4.04609254 | 1.00090614 |
| H | 0.00000000 | -4.04609254 | 1.00090614 |
| H | 1.65894780 | 2.42602225 | 3.43712000 |
| H | -1.65894780 | 2.42602225 | 3.43712000 |
| H | 1.65894780 | -2.42602225 | 3.43712000 |
| H | -1.65894780 | -2.42602225 | 3.43712000 |

## S3.49 Thioacrolein

| | | | |
|---|---|---|---|
| C | 4.27693177 | 0.00000000 | -0.88320133 |
| C | 1.76449030 | 0.00000000 | -1.23998444 |
| C | 0.00891877 | 0.00000000 | 0.85393278 |
| S | -3.06510749 | 0.00000000 | 0.58558716 |
| H | 5.57642075 | 0.00000000 | -2.45571463 |
| H | 5.06950243 | 0.00000000 | 1.00139499 |
| H | 0.96616458 | 0.00000000 | -3.11935314 |
| H | 0.87110201 | 0.00000000 | 2.71756937 |

## S3.50 Thioformaldehyde

Ground state

| | | | |
|---|---|---|---|
| C | 0.00000000 | 0.00000000 | -2.08677304 |
| S | 0.00000000 | 0.00000000 | 0.97251194 |
| H | 0.00000000 | 1.73657773 | -3.17013507 |
| H | 0.00000000 | -1.73657773 | -3.17013507 |

Excited state ($^1A_2$ state in the $C_{2v}$ point group)

| | | | |
|---|---|---|---|
| C | 0.00000000 | 0.00000000 | -2.20256705 |
| S | 0.00000000 | 0.00000000 | 1.02717172 |
| H | 0.00000000 | 1.76634191 | -3.21909384 |
| H | 0.00000000 | -1.76634191 | -3.21909384 |

## S3.51 Thiophene

| | | | |
|---|---|---|---|
| C | 0.00000000 | 2.33342542 | -0.09858421 |
| C | 0.00000000 | -2.33342542 | -0.09858421 |
| C | 0.00000000 | 1.34371718 | -2.48297725 |
| C | 0.00000000 | -1.34371718 | -2.48297725 |
| S | 0.00000000 | 0.00000000 | 2.17250692 |
| H | 0.00000000 | 4.29028016 | 0.44577296 |
| H | 0.00000000 | -4.29028016 | 0.44577296 |
| H | 0.00000000 | 2.48760051 | -4.16768392 |
| H | 0.00000000 | -2.48760051 | -4.16768392 |

## S3.52 Thiopropynal

| | | | |
|---|---|---|---|
| C | -0.00382924 | 0.00000000 | -1.25249909 |
| C | -2.27832423 | 0.00000000 | 0.15152736 |
| C | -4.26309583 | 0.00000000 | 1.29548793 |
| S | 2.81920288 | 0.00000000 | -0.00828974 |
| H | -0.23056990 | 0.00000000 | -3.28862183 |
| H | -5.97712967 | 0.00000000 | 2.33206931 |
